# Supplementary material for: Constant-Time Snapshots with Applications to Concurrent Data Structures
Source: arXiv:2007.02372 source file (2020-12-30)
Supplement: Supplementary file 1 [file ppopp-snapshot-submission-appendix.pdf]

## A Detailed Proof of Correctness of versioned CAS and camera Objects

### A.1 Linearization Points

Given a camera object  $S$  and a versioned CAS object  $O$  associated with it, in this section, we describe how their operations are linearized, but we defer the detailed proof of Theorem 2 to Appendix A.2.

To state the linearization points, we first introduce some useful terminology. When referring to the variables  $O.VHead$  and  $S.timestamp$ , we often abbreviate them to  $VHead$  and  $timestamp$ . We say that a  $VNode$  has a *valid* timestamp at some configuration  $C$  if the value of its  $ts$  field is not `TBD` at  $C$ . Otherwise, the timestamp of the node is called *invalid*. We use the term *version list* to refer to the list that results from starting at the  $VNode$  pointed to by  $VHead$  and following the `nextv` pointers. The *head* of the version list is the  $VNode$  pointed to by  $VHead$ .

The only way to modify the version list is the `CAS` at Line 46, which swings the  $VHead$  pointer to a new  $VNode$  whose `nextv` pointer points to the previous head of the version list. This has the effect of adding the new  $VNode$  to the beginning of the version list. Before this can happen, `initTS` is called to install a valid timestamp in the old head of the version list. This ensures that the only  $VNode$  in the version list with an invalid timestamp is the first one. At the time a  $VNode$ 's timestamp becomes valid, it is therefore still at the head of the version list.

The correctness of `readSnapshot` operations depends on ensuring that the timestamp associated with a value is current (i.e., in  $S.timestamp$ ) at the linearization point of the `vCAS` that stored the value in  $O$ . So, we linearize a `vCAS` that adds a  $VNode$  to the version list at the time that the timestamp eventually written into that  $VNode$  was read from  $S.timestamp$ . This means that there may be a  $VNode$  at the head of the version list before the `vCAS` that created that  $VNode$  is linearized. This is why any other operation that finds a  $VNode$  with an invalid timestamp at the head of the version list calls `initTS` to help install a valid timestamp in it before proceeding. This helping mechanism is crucial in the argument that all of the following linearization points are well-defined and within the intervals of their respective operations.

- A `vCAS` operation is linearized depending on how it executes.
  - If the `vCAS` performs a successful `CAS` on Line 46 that adds a node  $n$  to the version list, and  $n$ 's timestamp eventually becomes valid, then the `vCAS` is linearized on Line 21 of the `initTS` method that makes  $n$ 's timestamp valid. Note that this case includes all `vCAS` operations that return `true` at Line 48.

- Let  $h$  be the value of  $VHead$  at Line 41 of a `vCAS` operation. If the `vCAS` operation returns on Line 43 or 44, then it is linearized either at Line 41 if  $h$ 's timestamp is valid at that time, or the first step afterwards that makes  $h$ 's timestamp valid.
- Finally, consider a `vCAS(oldV, newV)` operation  $V$  that returns `false` on Line 52. This is the most subtle case. The return on Line 52 is only reached when  $V$  fails its `CAS` on Line 46 because some other `vCAS` operation changed  $VHead$  after  $V$  read it at Line 41. We linearize the `vCAS` immediately after the linearization point of the `vCAS` operation  $V'$  that made the *first* such change. (If several `vCAS` operations that return on Line 52 are linearized immediately after  $V'$ , they can be ordered arbitrarily.)
- For a `vRead` operation that terminates, let  $h$  be the  $VNode$  read from  $VHead$  at Line 37. The `vRead` is linearized at Line 37 if  $h$ 's timestamp is valid at that time, or at the first step afterwards that makes  $h$ 's timestamp valid.
- A `readSnapshot` operation that terminates is linearized at its last step.
- For `takeSnapshot` operations, let  $t$  be the value read from `timestamp` on line 5. A `takeSnapshot` operation that terminates is linearized when the value of `timestamp` changes from  $t$  to  $t + 1$ .

### A.2 Proof of Correctness

In this section, we prove that Fig. 1 is a linearizable implementation of versioned CAS and camera objects. First we argue that it suffices to prove linearizability for histories consisting of a single versioned CAS object and a single camera object. Suppose two versioned CAS objects are associated with different camera objects. Then we can prove linearizability for the two sets of objects independently because they do not access any common variables and do not affect each other in terms of sequential specifications. Suppose two versioned CAS objects  $O_1$  and  $O_2$  are associated with the same camera object  $S$ . Let  $H'$  be a history of operations on these three objects. Furthermore, let  $H'_1$  be the history  $H'$  restricted to only operations from  $S$  and  $O_1$ , and similarly, let  $H'_2$  be the history  $H'$  restricted to only operations from  $S$  and  $O_2$ . We will define the linearization points of  $S$  so that they are not affected by operations on  $O_1$  or  $O_2$ . Therefore, showing that both  $H'_1$  and  $H'_2$  are linearizable is sufficient for showing that  $H'$  is linearizable because  $S$  will be linearized the same way in both  $H'_1$  and  $H'_2$ .

Let  $H$  be a history of a versioned CAS object  $O$  and a camera object  $S$ . We assume that  $S$  and  $O$  are initialized by their constructors (Line 3 and 15, respectively) before the beginning of  $H$ . We assume this history satisfies the precondition (described in Definition 1) that whenever `readSnapshot(ts)` is invoked, there must be a completed `takeSnapshot` operation that returned  $ts$ . When referring to the variables

`O.VHead` and `S.timestamp`, we will often abbreviate them to `VHead` and `timestamp`.

We first introduce some useful terminology. We say that a `VNode` has a *valid* timestamp at some configuration  $C$  if the value of its `ts` field is not `TBD` at  $C$ . Otherwise, the timestamp of the node is called *invalid*. We use the term *version list* to refer to the list that results from starting at the `VNode` pointed to by `VHead` and following the `nextv` pointers. The *head* of the version list is the `VNode` pointed to by `VHead`.

A *modifying* `vCAS` operation is one that performs a successful CAS on line 46. Due to the if statement on line 44, if `vCAS(oldV, newV)` is a modifying `vCAS` operation, then `oldV`  $\neq$  `newV`. Note that modifying `vCAS` operations can return only on line 48 and any operation that returns on line 48 is a modifying `vCAS`. A `vCAS` is *successful* if it is a modifying `vCAS` or if it returns `true` at line 44. Otherwise, it is *unsuccessful*.

We first show that the only change to a version list is inserting a `VNode` at the beginning of it.

**Lemma 3.** *Once a `VNode` is in the version list, it remains in the version list forever.*

*Proof.* The only way to change a version list is a successful CAS at line 46, which changes `VHead` from `head` to `newN`. When this happens, `newN->nextv` = `head`, so all `VNodes` that were in the version list before the CAS are still in the version list after the CAS.  $\square$

It is easy to check that every time we access some field of an object via a pointer to that object, the pointer is not `NULL`. `VHead` always points to a `VNode` after it is initialized on Line 17 of  $O$ 's constructor. It follows that every call to `initTS` is on a non-null pointer. The precondition of `readSnapshot(ts)` ensures that `ts` is a timestamp obtained from  $S$  after  $O$  was initialized and is therefore greater than or equal to the timestamp that  $O$ 's constructor stored in the initial `VNode` of the version list. Thus, the `readSnapshot` will stop traversing the version list when it reaches that initial `VNode`, ensuring that node is never set to `NULL` on line 34.

#### Linearization Points.

Before we can define the linearization points, we need a few simple lemmas that describe when `VNodes` have valid timestamps. We start with an easy lemma about `initTS`.

**Lemma 4.** *The following hold:*

1. *Before `initTS` is called on a `VNode`, `VHead` has contained a pointer to that `VNode`.*
2. *After a complete execution of `initTS` on some `VNode`, that `VNode`'s timestamp is valid.*

*Proof.* All calls to `initTS` are done on a pointer that has either been read from `VHead` or successfully CASed into `VHead`. Once a timestamp is valid, it can never be modified again, since only a CAS on line 22 modifies the `ts` variable of any `VNode`. The CAS on Line 22 can fail only if the `ts` variable is already a valid timestamp.  $\square$

**Lemma 5.** *In every configuration  $C$ , the only `VNode` in the version list that can have an invalid timestamp is the head of the version list.*

*Proof.* No `VNode`'s `nextv` pointer changes after the `VNode` is created, so the only way the version list can change is when `VHead` is updated. Moreover, no `VNode`'s timestamp ever changes from valid to invalid. So, we must only show that updates to `VHead` preserve the claim.

The value of `VHead` changes only when a successful CAS is executed on Line 46 of an instance of `vCAS`. Consider any such successful CAS by some process  $p$  and assume the claim holds in the configuration before the CAS to show that it holds immediately after the CAS. This CAS changes `VHead` from `head` to `newN`. By the initialization of `newN` on Line 45, that `VNode`'s `nextv` pointer is `head`. So, we must show that `head` and all `VNodes` reachable from `head` by following `nextv` pointers have valid timestamps when the CAS occurs. Before executing this CAS,  $p$  executes `initTS(head)`, so, by Lemma 4(2), that `VNode`'s timestamp is valid at the time that the CAS is executed. Since the CAS is successful, `VHead` was equal to `head` immediately before the CAS, so all nodes reachable from that `VNode` had valid timestamps, by our assumption.  $\square$

The next lemma is used to define the linearization point of a modifying `vCAS`.

**Lemma 6.** *Suppose an invocation of `initTS` makes the timestamp of some `VNode`  $n$  valid. Then,  $n$  is the head of the version list when that `initTS` executes Line 21 and 22.*

*Proof.* By Lemma 4(1), every call to `initTS` is on a pointer that has previously been in `VHead`, so  $n$  has been in the version list before `initTS` is called. By Lemma 3,  $n$  is still in the version list when Line 21 and 22 are executed. By Lemma 5,  $n$  remains at the head of the version list until its timestamp becomes valid when `initTS` performs Line 22.  $\square$

We are now ready to define linearization points. As we define them, we argue that the linearization point of each operation is well-defined and within the interval of the operation.

- A `vCAS` operation is linearized depending on how it executes.
  - If the `vCAS` performs a successful CAS on Line 46 that adds a node  $n$  to the version list, and  $n$ 's timestamp eventually becomes valid, then the `vCAS` is linearized on Line 21 of the `initTS` method that makes  $n$ 's timestamp valid. Lemma 6 implies that the linearization point occurs after the `vCAS` adds  $n$  to the version list at Line 46. If the `vCAS` terminates, it first calls `initTS` on  $n$  at line 47, so Lemma 4(2) ensures the `vCAS` is linearized and that the linearization point comes before the end of that `initTS`.

- Let  $h$  be the value of  $VHead$  at Line 41 of a  $vCAS$  operation. If the  $vCAS$  operation returns on Line 43 or 44, then it is linearized either at Line 41 if  $h$ 's timestamp is valid at that time, or the first step afterwards that makes  $h$ 's timestamp valid. Lemma 4(2) ensures this step exists and is within the interval of the  $vCAS$ , since  $initTS$  is called on  $h$  at line 42.
  - Finally, consider a  $vCAS(oldV, newV)$  operation  $V$  that returns `false` on Line 52. This is the most subtle case. The return on Line 52 is only reached when  $V$  fails its CAS on Line 46 because some other  $vCAS$  operation changed  $VHead$  after  $V$  read it at Line 41. We linearize the  $vCAS$  immediately after the  $vCAS$  operation  $V'$  that made the *first* such change. (If several  $vCAS$  operations that return on Line 52 are linearized immediately after  $V'$ , they can be ordered arbitrarily.)
- To argue that this linearization point is well-defined, we must show that the  $VNode$   $n$  that  $V'$  added to the version list gets a valid timestamp, so that  $V'$  is assigned a linearization point as described in the first paragraph above. By Lemma 3,  $n$  is still in the version list when  $V$  reads  $VHead$  at Line 51. If  $n$  is no longer at the head of the version list, then  $n$ 's timestamp must be valid, by Lemma 5. Otherwise, if  $n$  is still the head of the version list, then  $n$ 's timestamp is guaranteed to be valid after  $V$  calls  $initTS$  on  $n$  (Line 51), by Lemma 4(2). So, in either case,  $V'$  is assigned a linearization point, which is before the timestamp of  $n$  becomes valid. Thus,  $V'$  (and therefore  $V$ ) is linearized before the end of  $V$ . Lemma 6 implies that the linearization point of  $V'$  (and therefore of  $V$ ) is after  $V'$  adds  $n$  to the version list, which is after  $V$  reads  $VHead$ . This proves that  $V$ 's linearization point is inside the interval of  $V$ .
- For a  $vRead$  operation that terminates, let  $h$  be the  $VNode$  read from  $VHead$  at Line 37. The  $vRead$  is linearized at Line 37 if  $h$ 's timestamp is valid at that time, or at the first step afterwards that makes  $h$ 's timestamp valid. Lemma 4(2) ensures that this step exists and is during the interval of the  $vRead$ , since the  $vRead$  calls  $initTS$  on  $h$  at Line 38.
  - A  $readSnapshot$  operation that terminates is linearized at its last step.
  - For  $takeSnapshot$  operations, let  $t$  be the value read from `timestamp` on line 5. A  $takeSnapshot$  operation that terminates is linearized when the value of `timestamp` changes from  $t$  to  $t + 1$ . We know that this occurs between the execution of Line 5 and 6: either the  $takeSnapshot$  operation made this change itself if the CAS at line 6 succeeds, or some other  $takeSnapshot$  operation did so, causing the CAS on line 6 to fail.

Note that all operations that terminate are assigned linearization points. In addition, some  $vCAS$  operations that do not terminate are assigned linearization points.

**Proof that Linearization Points are Consistent with Responses** Recall that  $H$  is the history that we are trying to linearize. In the rest of this section, we prove that each operation returns the same response in  $H$  as it would if the operations were performed sequentially in the order of their linearization points.

**Lemma 7.** Assume  $VHead$  points to a node  $h$  in some configuration  $C$ . If  $h.ts$  is valid in  $C$  then either  $h$  is the  $VNode$  created by the constructor of  $O$ , or the  $vCAS$  that created  $h$  is linearized before the configuration that immediately precedes  $C$ .

*Proof.* Suppose  $h.ts$  is valid in  $C$  but  $h$  is not the  $VNode$  created by the constructor of  $O$ . Then  $h$  is created by some  $vCAS$  operation  $V$  that added  $h$  to the head of the version list. Since  $h.ts$  is valid in  $C$ , some step prior to  $C$  set  $h.ts$  by executing Line 22. The linearization point of  $V$  is at the preceding execution of Line 21. Thus, the linearization point precedes the configuration before  $C$ .  $\square$

We define the *value of the versioned CAS object in configuration  $C$*  to be the value that a versioned CAS object would store if all of the  $vCAS$  operations linearized before  $C$  are done sequentially in linearization order (starting from the initial value of the versioned CAS object). The following crucial lemma describes how the value of the versioned CAS object is represented in our implementation. It also says that the responses returned by all  $readSnapshot$  and  $vCAS$  operations are consistent with the linearization points we have chosen.

**Lemma 8.** In every configuration  $C$  of  $H$  after the constructor of the versioned CAS object has completed,

1. if  $VHead$  points to the  $VNode$  created by the constructor of the versioned CAS object, then  $VHead \rightarrow val$  is the value of the versioned CAS object,
2. if the linearization point of the  $vCAS$  that created the first node in the version list is before  $C$ , then  $VHead \rightarrow val$  is the value of the versioned CAS object, and
3. otherwise,  $VHead \rightarrow nextv \rightarrow val$  is the value of the versioned CAS object.

Moreover, each  $vRead$  and  $vCAS$  operation that is linearized at or before  $C$  returns the same result in  $H$  as it would return when all operations are performed sequentially in their linearization order.

*Proof.* We prove this by induction on the length of the prefix of  $H$  that leads to  $C$ . In the configuration immediately after the constructor of the versioned CAS object terminates,  $VHead \rightarrow val$  stores the initial value of the versioned CAS object.



Since `nextV` and `val` fields of a `VNode` do not change after the `VNode` is created, we must only check that the invariant is preserved by steps that modify `VHead` or are linearization points of `vCAS` operations (which may change the value of the versioned CAS object) or `vRead` operations. We consider each such step  $s$  in turn and show that, assuming the claim holds for the configuration  $C$  before  $s$ , then it also holds for the configuration  $C'$  after  $s$ .

First, suppose  $s$  is a successful CAS on `VHead` at line 46 of a `vCAS` operation. It changes `VHead` from `head` to `newN`, where `newN->next = head`. By Lemma 5, `head->ts` is valid when this CAS occurs, since `head` becomes the second node in the version list. By our assumption, the value of the versioned CAS object prior to the CAS is `head->val`. Since this step is not the linearization point of any `vCAS` operation, the value after the CAS is still `head->val`. By Lemma 4(1) `initTS` is only called on a pointer that has been in `VHead` previously, and `newN` has never been in `VHead` before this CAS, we know that `newN->ts` is TBD. So the invariant holds after the CAS, since `VHead->nextV->val = head->val`.

Now, consider a step  $s$  that is the linearization point of a modifying `vCAS`(`oldV`, `newV`), which we denote  $V$ , possibly followed by the linearization points of some other `vCAS` operations that return `false` on Line 52. Since  $V$  is a modifying `vCAS`, it added a new `VNode`  $n_1$  to the head of the version list in front of node  $n_2$ . This happens after  $V$  checks that `n2.val = oldV  $\neq$  newV` on Line 43–44 and sets `n1.nextV` to point to  $n_2$  and sets `n1.val` to `newV` on Line 45. By Lemma 6,  $n_1$  is still the head of the version list when step  $s$  occurs. So in the configuration  $C$  before  $s$ , the value in the versioned CAS object is `n2.val = oldV`, by our assumption that the claim holds in  $C$ . Thus, when  $V$  occurs in the sequential execution, it returns `true` and changes the value of the versioned CAS object to `newV`. Note that `VHead->val = newV` in  $C'$ . It remains to check that all other `vCAS` operations that return `false` at line 52 and are linearized immediately after  $V$  should return `false` in the sequential execution and therefore do not change the value of the versioned CAS object. Consider any such `vCAS`  $V'$  of the form `vCAS`(`oldV'`, `newV'`). By the definition of the linearization point of  $V'$ ,  $V$  makes the first change to `VHead` after  $V'$  reads it on Line 41. So,  $V'$  must have read a pointer to  $n_2$  on Line 41. Since  $V'$  returns `false` at Line 52, it must have seen `n2.val = oldV'` at Line 43. Thus, `oldV' = n2.val = oldV  $\neq$  newV`, so when each of the `vCAS` operations  $V'$  is executed sequentially in linearization order, it should return `false` and leave the state of the versioned CAS object equal to `newV`. The claim for  $C'$  follows.

Finally, consider a step  $s$  that is the linearization point of one or more `vRead` operations or `vCAS` operations that return at Line 43 or 44. Consider any such operation  $op$ . Let  $h$  be the node at the head of the version list when  $op$  reads `VHead` at Line 37 or 41. Then  $s$  is either this read or a subsequent execution of Line 22 that makes  $h$ 's timestamp

valid. Either way, `VHead` points to  $h$  in  $C'$ , by Lemma 6. By Lemma 7, either case (1) or (2) of the claim applies to configuration  $C$ . Either way, the value of the versioned CAS object in  $C$  is `h.val`. If  $op$  is a `vRead`, then it returns `h.val` as it should. If  $op$  is a `vCAS` that returns `false` at Line 43, it would do the same in the sequential execution in linearization order because  $op$  reads the state of the versioned CAS object in  $C'$  from `h.val` on Line 43 and sees that it does not match its `oldV` argument. If  $op$  returns `true` at Line 44, it would also return `true` when performed in linearization order because the state of the versioned CAS object in  $C'$  matches both  $op$ 's `oldV` and `newV` values. In all cases the value of the versioned CAS object does not change as a result of  $op$ , so it is still `h.val` in  $C'$ , and the invariant is preserved.  $\square$

The following observation follows directly from the way modifying `vCAS` operations are linearized.

**Observation 9.** Consider a `VNode`  $n$  that was added to the version list by a modifying `vCAS`  $V$ . If the timestamp of  $n$  is valid, then `n.ts` stores the value of  $S$ . timestamp at the linearization point of  $V$ .

The following key lemma asserts that version lists are properly sorted.

**Lemma 10.** The modifying `vCAS` operations are linearized in the order they insert `VNodes` into the version list.

*Proof.* Consider any two consecutive `VNodes`  $n_1$  and  $n_2$  in the version list, where  $n_1$  is inserted into the list before  $n_2$ , and let  $V_1$  and  $V_2$  be the `vCAS` operations that inserted  $n_1$  and  $n_2$  to the list, respectively. Recall that the linearization point of a modifying `vCAS` is at the read of the timestamp (Line 21) of the `initTS` call that validates the timestamp on the `VNode` that this `vCAS` appended to the version list. In particular, a modifying `vCAS` is linearized after it inserts its `VNode` into the list (since `initTS` cannot be called on a `VNode` before it is inserted, by Lemma 4(1)), but before its `VNode` is assigned a valid timestamp on Line 22 of `initTS`. By Lemma 5, a `VNode` is assigned a valid timestamp before it is replaced as the head of the version list. That is,  $V_1$  must be linearized before  $n_1$ 's timestamp was valid, and  $n_1$ 's timestamp became valid before  $n_2$  was added to the list. Furthermore,  $V_2$  was linearized after  $n_2$  was added to the list. Therefore,  $V_1$  is linearized before  $V_2$ .  $\square$

Now, we prove our main theorem which says that our versioned CAS and camera algorithms are linearizable and have the desired time bounds.

*Proof (Theorem 2).* We show that the return values of each operation is correct with respect to their linearization points. For `vCAS` and `vRead` operations, this follows from Lemma 8.

We prove this for `takeSnapshot` and `readSnapshot` simultaneously. Suppose a `S.takeSnapshot` operation  $T$

returns a timestamp  $t$ , which is passed into a  $O.readSnapshot$  operation  $R$ . We show that  $R$  returns the value of  $O$  at the linearization point of  $T$ . Let  $h$  be the value of  $vHead$  on line 32 of  $R$ . The timestamp of  $h$  is valid after line 33 of  $R$ , and by Lemma 5, the timestamps of all the nodes in the version list starting from  $h$  are valid. This means that on line 34,  $node \rightarrow ts$  is never TBD. Let  $n$  be the value of  $node$  at the last line of  $R$  and let  $V$  be the modifying  $vCAS$  operation that appended  $n$ . We know that  $n$  is the first node in the version list starting from  $h$  with timestamp less than or equal to  $t$ . Since  $T$  is linearized when  $S.timestamp$  gets incremented from  $t$  to  $t + 1$ , by Observation 9,  $V$  is linearized before the linearization point of  $T$ . Since  $R$  returns the value written by  $V$ , it suffices to show that no modifying  $vCAS$  operation gets linearized between the linearization points of  $V$  and  $T$ . By Lemma 10, modifying  $vCAS$  operations are linearized in the order they appended  $vNodes$  to the version list. Therefore, for all nodes that are older than  $n$  in the version list, their modifying  $vCAS$  operations are linearized before the linearization point of  $V$ . Next, we show that all nodes in the version list that are newer than  $n$  are linearized after  $T$ . From the while loop on line 34, we can see that all nodes that lie between  $h$  and  $n$  (including  $h$ , excluding  $n$ ) have timestamps are larger than  $t$ . All nodes in the version list that are newer than  $h$  also have timestamp larger than  $t$  because they are appended after line 32 of  $R$  and  $S.timestamp$  is already greater than  $t$  at this step. Therefore, by Observation 9, all nodes in the version list newer than  $n$  are linearized after the linearization point of  $T$ . This means  $V$  is the last modifying  $vCAS$  operation to be linearized before the linearization point of  $T$ , as required.

The bounds on the step complexity of the operations can be derived trivially by inspection of the pseudocode.  $\square$

## B Adding Linearizable Queries to Concurrent Data Structures

In this section, we show how to use versioned CAS objects to extend a large class of concurrent data structures that are implemented using reads and CAS primitives to support linearizable wait-free queries. Throughout the section we also use NBBST as an example to show how our approach works. The idea of this construction is to replace CAS objects with their versioned counterparts, and to use this to obtain *snapshots* of the concurrent data structure. We can then run queries on the obtained snapshot, without worrying about concurrent updates to the data structure.

The techniques in this section are general. For many data structures, they allow translating any read-only operation on a sequential data structure into a linearizable query on the corresponding concurrent data structure. To achieve this generality, the techniques go through multiple layers of abstraction. To make it more concrete, we show examples of how to add specific linearizable queries to the Michael and Scott queue [42] and NBBST tree [26] in Appendix E.

We present this construction in two parts. First, we define the concept of *solo linearizable* queries. A *query* operation is an operation that does not modify the shared state (i.e., it is read-only). A *solo linearizable query* (or *solo query*) is a query operation that is only guaranteed to be correct if it is run solo. Intuitively, a solo query is one that can run on a “snapshot” of a concurrent data structure, and it never changes the current state of the data structure. They may be invoked while other operations are pending, but once invoked, they need to run to completion without any other process taking steps during their interval. Section B.1 describes how to transform a concurrent data structure that supports solo queries (which we refer to as a *solo linearizable* data structure) into a fully linearizable one using our versioned CAS objects. However, most concurrent data structures in the literature do not come with solo queries. In Section B.2, we discuss how to add solo query operations to a given linearizable data structure.

**Definition 11.** We denote by  $\mathcal{H}(D, Q)$  the set of histories of concurrent data structure  $D$  in which every operation instance from some set of query operations  $Q$  is run solo.

**Definition 12.** A concurrent data structure  $D$  is *linearizable with solo queries*  $Q$  if every history  $H \in \mathcal{H}(D, Q)$  is linearizable. A query  $q \in Q$  is called a *solo linearizable* query on  $D$ . With clear context of solo queries  $Q$ , we call  $D$  a *solo linearizable data structure*.

The running time of a solo query may depend on the concurrent state at which it is run. We denote by  $T(q, C)$  the running time (number of steps) of a solo query  $q$  at concurrent state  $C$  of the data structure.

### B.1 Making Solo Queries Fully Linearizable

We now show how to transform a solo linearizable data structure  $D$ , implemented with CAS objects, that has a set of solo queries  $Q_D$ , into a fully linearizable data structure  $D_\ell$ . Let  $L_D$  be the operations of  $D$  that are not in  $Q_D$ . The transformation uses our versioned CAS objects in place of the regular CAS objects of  $D$ . It preserves all existing correctness guarantees (e.g., linearizability, strong linearizability, sequential consistency) and progress guarantees (e.g., wait-freedom, lock-freedom) of the operations in  $L_D$ . Furthermore, it preserves the running time of operations of  $L_D$  up to constant factors. The time complexity of a linearizable query  $q \in Q_D$  in  $D_\ell$  is bounded by  $q$ 's time complexity in  $D$ , plus a contention term.

**Construction 13.** To obtain  $D_\ell$  we replace every CAS object with a versioned CAS object, initialized with the same value. All versioned CAS objects are associated with a single camera object. Each CAS or read by an operation in  $L_D$  on a CAS object is replaced by a  $vCAS$  or  $vRead$  (respectively) on the corresponding versioned CAS object. To perform a solo query operation  $q \in Q_D$  in  $D_\ell$ , a process  $p$  first

executes `takeSnapshot` on the camera object, to obtain a handle  $h$ . Then, for any CAS object in  $D$  that  $q$  would have accessed,  $p$  performs `readSnapshot( $h$ )` on the corresponding versioned CAS object. Recall that all operations in  $Q_D$  are read-only, and thus never perform a CAS.

For this construction to be legal, we must show that the precondition for `readSnapshot( $h$ )` holds. Namely, we need to show that `readSnapshot( $h$ )` is never called on a versioned CAS object that was created after the handle  $h$  was produced. Intuitively, this is satisfied since no versioned CAS object that was created after  $h$  can be reachable in the data structure through version nodes with timestamp  $h$  or earlier, which are the only version nodes that a query reads. The following claim makes the argument more formal.

**Claim 14.** *In Construction 13, no versioned CAS object  $O$  is ever accessed using a `readSnapshot( $h$ )` operation where  $h$  was produced before  $C$  was created.*

*Proof.* Consider a query operation  $q \in Q_D$  that uses handle  $h$  to run on a data structure  $D_\ell$  as prescribed by Construction 13. We say that a versioned CAS object is *new* if it was created after  $h$  was produced, and *old* otherwise. Assume by contradiction that  $q$  accesses a new  $\text{vCAS}$  object  $O_{\text{new}}$ .  $O_{\text{new}}$  must be reachable from the root of  $D_\ell$  for  $q$  to access it. Note that by the way  $D_\ell$  is initialized, the root must be an old versioned CAS object. Without loss of generality, assume  $O_{\text{new}}$  is the first new object that  $q$  accesses in its execution.  $O_{\text{new}}$  must be pointed to by some old versioned CAS object  $O_{\text{old}}$ , through which  $q$  accessed  $O_{\text{new}}$ . Since the only updates to versioned CAS objects are via  $\text{vCAS}$  operations,  $O_{\text{old}}$  must have been updated with a  $\text{vCAS}$  to point to  $O_{\text{new}}$ , thereby creating a new version of  $O_{\text{old}}$ . Note that since  $O_{\text{new}}$  was created after  $h$ , this update must have also happened after  $h$  was produced, and therefore the version of  $O_{\text{old}}$  that points to  $O_{\text{new}}$  has a timestamp larger than  $h$ . So,  $q$  executing `readSnapshot( $h$ )` on  $O_{\text{old}}$  would not access the version pointing to  $O_{\text{new}}$ , but some older version instead. This contradicts the fact that  $q$  reaches  $O_{\text{new}}$ .  $\square$

Using Construction 13, we can make solo queries linearizable with the bounds specified in the following theorem.

**Theorem 15.** *Given a concurrent data structure  $D$  with a set of linearizable operations  $L_D$  and a set of solo query operations  $Q_D$ . Construction 13 produces a linearizable data structure  $D_\ell$  that supports operations from both  $L_D$  and  $Q_D$ . This construction maintains the following properties:*

- Operations from  $L_D$  have the same progress properties in  $D_\ell$  as in  $D$ , and their runtimes are increased by only a constant factor.
- Each operation  $q \in Q_D$  costs  $O(T(q, C_\ell) + W \cdot A)$  where  $C_\ell$  is the concurrent state at which  $q$  executes the `takeSnapshot` operation,  $W$  is the number of  $\text{vCAS}$  operations concurrent with  $q$  on memory locations accessed by  $q$  in the execution, and  $A$  is the maximum

number of repeated accesses to the same object by the query.

The proof is in Appendix C. We note that in most cases, the number of accesses that a query executes to the same object is 1 (or a small constant). If not, this bound can be improved by caching the values read from the data structure locally to avoid the extra overhead of reading it repeatedly from the concurrent data structure.

## B.2 Adding Solo Queries to Linearizable Data Structures

Concurrent data structures in the literature are usually designed to support a set of operations that are all linearizable. Thus, the question of whether solo linearizable operations can be easily incorporated is generally not considered when designing these data structures. Is it always possible to run queries in a linearizable manner on a snapshot of any given data structure? How efficient can such queries be? In this section, we address these questions.

While designing queries to run solo is certainly much simpler than designing them to be linearizable in the concurrent setting, it is still not as easy as designing queries for a sequential data structure. This is because, in some cases, linearization points cannot be uniquely determined from the state of shared memory; instead, the linearization points may only be determined at the end of the execution, since they can depend on future events. If this is the case, a query that is run solo cannot determine whether a pending update operation has linearized or not, and, since the query may not change the state, it cannot enforce a placement of the linearization point. Herlihy and Wing [36] describe a queue implementation in which the linearization order of the enqueue operations depends on future dequeue operations. For that algorithm, no solo query is possible. Herlihy and Wing [36] point out that the difficulty in this scenario is the absence of an *abstraction function* from states of the implementation to states of the abstract data type being implemented. We therefore define the notion of *direct linearizability*, which intuitively means that there is always such a mapping from every concurrent state in an execution of the concurrent data structure to the abstract state of the abstract data type being implemented.

**Definition 16.** An *abstraction function* of a solo linearizable data structure  $D$  with solo queries  $Q$  that implements an abstract data type  $A$ , is a function  $F : C_D \rightarrow C_A$  from concurrent states of  $D$  to abstract states of  $A$  such that for every history  $H \in \mathcal{H}(D, Q)$ , there exists a linearization of  $E$  such that:

1.  $F$  maps the initial state of  $D$  to the initial state of  $A$  (i.e.,  $F(C_D^{\text{init}}) = C_A^{\text{init}}$ ).
2. If a concurrent state of  $D$ ,  $C_{D,2}$  can be obtained from another concurrent state  $C_{D,1}$  in  $H$  without the linearization of any operation between  $C_{D,1}$  and  $C_{D,2}$ , then they map to the same abstract state (i.e.,  $F(C_{D,1}) = F(C_{D,2})$ ).



3. If a concurrent state of  $D$ ,  $C_{D,2}$  can be obtained from another concurrent state  $C_{D,1}$  in  $H$  where operations,  $op_1, \dots, op_k$ , linearized between  $C_{D,1}$  and  $C_{D,2}$  in this order, then  $F(C_{D,2})$  is the state of  $A$  that is obtained from applying  $op_1 \dots op_k$  in this order to  $F(C_{D,1})$ .

Intuitively, the abstraction function respects the linearization points in the execution of  $D$ . At first glance, it seems like the abstraction function's behavior is determined solely by the update operations from  $D$ . However, query operations do have an indirect impact because they can affect the linearization points of the update operations, which affects the behavior of the abstraction function. When the definition is applied to fully linearizable data structures,  $Q = \emptyset$ , so  $\mathcal{H}(D, Q)$  is the set of all histories of  $D$ .

**Definition 17.** A linearizable data structure is said to be *directly linearizable* if it has an abstraction function.

Direct linearizability is reminiscent of *strong linearizability* [34]. Strong linearizability requires that the linearizations can be chosen for histories in a *prefix-preserving* way: for a prefix  $H_p$  of a history  $H$ , the linearization of  $H_p$  must be a prefix of the linearization of  $H$ . Thus, future events cannot determine whether a given step in the execution was a linearization point or not. Intuitively, direct linearizability requires that update operations be strongly linearizable, but does not require the same behavior from query operations (that do not change the high-level state). Furthermore, while strong linearizability only requires this “prefix preserving” behavior for parts of the state that can be observed by operations of the data structure, direct linearizability imposes this behavior on the entire shared state, regardless of the interface through which operations of the data structure can access it. Appendix D shows that strong and direct linearizability are incomparable. However, all strongly linearizable data structures that we are aware of are also directly linearizable.

Consider the NBBST binary search tree [26] outlined in Section 4. Recall that NBBST implements the *ordered set* abstract data type, with keys as elements. To avoid special cases, the tree includes two leaves containing dummy keys.

**Proposition 18.** Consider the function  $F : C_E \rightarrow C_A$  that maps concurrent states of the NBBST BST to states of the ordered set abstract data type as follows. Given a concurrent state  $C_E$  of NBBST,  $F(C_E)$  is the set of keys in leaf nodes reachable from the root in  $C_E$  except for the two dummy keys.  $F$  is an abstraction function of NBBST.

*Proof.* This theorem is proved as Lemmas 29 and 30 in the technical report [26], so we just sketch it here. Initially, the tree has only the two leaves containing the dummy keys, which  $F$  maps to the empty set, as desired. Each  $\text{Insert}(k)$  that modifies the tree is linearized at the child CAS that adds a leaf containing  $k$  to the tree (and it is shown that  $k$  was not present in the tree before this change). Similarly, each  $\text{Delete}(k)$  that modifies the tree is linearized at the child

CAS that removes a leaf containing  $k$  from the tree. Each  $\text{Insert}(k)$  that returns `false` is linearized when  $k$  is in a leaf of the tree, and each  $\text{Delete}(k)$  that returns `false` is linearized when there is no leaf containing  $k$ , so these operations have no effect on the tree or on the abstract state of the set. Each terminating  $\text{Find}(k)$  returns `true` if and only if  $k$  appears in some leaf at the linearization point of the  $\text{Find}$ . It follows that each operation is linearized so that its effect on the set of keys stored in leaves exactly matches its effect on the abstract state of the ordered set that the tree implements.  $\square$

Abstraction functions can help us both design solo queries and prove their correctness. It is often helpful to reason about solo queries based on how they behave on each concurrent state. For this purpose, we present the following definition.

**Definition 19.** Let  $op$  be an operation from a concurrent data structure  $D$  and let  $C$  be a reachable concurrent state, we define  $op(C)$  to be the response value of  $op$  when run solo on concurrent state  $C$ .

Now we present a proof technique for showing that a read-only operation  $q$  is a solo query. Consider a concurrent data structure  $D$  that implements an abstract data type  $A$  and is linearizable with solo queries  $Q$ . Suppose  $D$  has an abstraction function  $F$ . We add a query operation  $q_A$  to  $A$  to get the ADT  $A'$  and we add  $q$  to  $D$  to get  $D'$ . Our goal is to show that  $D'$  is an implementation of  $A'$  that is linearizable with solo queries  $Q \cup \{q_A\}$ . The following observation says that it suffices to show  $q(C) = q_A(F(C))$  for all reachable concurrent states  $C$ .

**Observation 20.** If  $q(C) = q_A(F(C))$  for any reachable concurrent state  $C$ , then  $D'$  is an implementation of  $A'$  that is linearizable with solo queries  $Q \cup \{q_A\}$ . Furthermore, in this case,  $F$  is still an abstraction function for  $D'$ .

Note that the set of reachable concurrent states for  $D$  does not change when we add a read-only operation  $q_A$  to  $D$ . The fact that  $F$  is still an abstraction function for  $D'$  is important because it allows us add solo queries one at a time. This is summarized by the following observation.

**Observation 21.** Suppose two data structures have the exact same linearizable operations  $L$ , but different solo queries  $Q_1$  and  $Q_2$ . If the same abstraction function works for both queries, then adding  $Q_2$  to the first data structure results in a new data structure that is linearizable with solo queries  $Q_1 \cup Q_2$ .

Next, we show how to use the abstraction function as a guide for designing solo queries. If the abstraction function is computable and there is some way of viewing/traversing the state of shared memory, then an easy, but not necessarily efficient, method would be to first traverse the state of  $D$ , then use the abstraction function to arrive at an abstract state, and finally compute the query on the abstract state. This query

literally computes  $q_A(F(C))$ , so we can apply Observation 20. This is inefficient, since traversing the entire concurrent state often takes much longer than executing the query. We show examples of how to compute queries designed for a sequential version of the data structure on a concurrent state.

**B.2.1 Solo queries for NBBST** Consider the NBBST. The concurrent state of the NBBST includes a lot of information used to coordinate concurrent updates. By removing everything except the root pointer, the `key`, `left`, `right` fields of each `Internal` node, and the `key` fields of each `Leaf` node, we end up with a standard leaf-oriented BST (with child pointers, but no parent pointers). This means that sequential read-only queries that work on a leaf-oriented BST, such as predecessor or range queries, can be run on the NBBST as is, because they only access fields that we keep. In the following theorem, we show that these read-only queries can be added to the NBBST as solo queries without any modification.

**Theorem 22.** *Let  $Q$  be a set of read-only, sequential operations on a leaf-oriented BST implementing a set of abstract queries  $Q_A$ . Let  $A'$  be an ADT that supports ordered set operations as well as queries from  $Q_A$ . Adding the operations in  $Q$ , without modification, to the NBBST yields a concurrent implementation of  $A'$  that is linearizable with solo queries  $Q$ .*

*Proof.* Let  $F$  be the abstraction function from Proposition 18 for NBBST. Pick any  $q \in Q$  and let  $q_A \in Q_A$  be the abstract operation that it implements. Our goal is to show that  $q(C) = q_A(F(C))$  for all reachable concurrent states  $C$ . Then we can apply Observations 20 and 21 to complete the proof.

We begin by defining a mapping  $F_A$  from states of leaf-oriented BSTs to states of  $A$  and a mapping  $F_I$  from concurrent states to states of a leaf-oriented BST. (The  $I$  in  $F_I$  stands for intermediate state because it is in between the abstract state and the concurrent state.) For  $F_A$  we use the textbook mapping which maps an leaf-oriented BST to the set of keys that appear in its leaves. Given an leaf-oriented BST state  $S$ , return value of  $q$  on state  $S$  (denoted  $q(S)$ ) equals  $q_A(F_A(S))$ . To compute the mapping  $F_I$ , we start with a concurrent state and remove everything except the root pointer, the `key`, `left`, `right` fields of each `Internal` node, and the `key` fields of each `Leaf` node. Since  $q$  only accesses the fields that we keep, it cannot tell the difference between running on a concurrent state  $C$  and running on  $F_I(C)$ . Therefore  $q(C) = q(F_I(C))$ . It is easy to verify that  $F = F_A \circ F_I$  and this completes the proof because  $q(C) = q(F_I(C)) = q_A(F_A(F_I(C))) = q_A(F(C))$ .  $\square$

We apply Construction 13 on top of Theorem 22 to get a data structure  $D_\ell$  that supports `insert`, `delete`, and `find`, as well as linearizable implementations of any query for which there is a read-only sequential algorithm. By Theorem 15, we maintain the efficiency of `insert`, `delete`, and `find` up to constant factors and for each new query operations in  $D_\ell$ , it is wait-free and its runtime is proportional to the sequential cost of the query plus  $W \cdot A$ , where  $W$  is the

number of `vCAS` operations that occur during the query and that operate on objects accessed by the query, and  $A$  is the maximum number of repeated accesses to the same object by the query. Most read-only, sequential operations on a leaf-oriented BST, such as `predecessor` and `range_query`, can be written so that each query accesses a memory location no more than a constant number of times. For such operations, the added cost is just  $O(W)$ . For example, consider a `range_query` operation that computes the list of keys within a certain range. If we start with a sequential implementation that takes  $O(h + k)$  time, where  $h$  is the height of the BST and  $k$  is the number of keys within the specified range, then the corresponding concurrent query in  $D_\ell$  would take  $O(h' + k + W)$  time, where  $h'$  is the height of the concurrent tree at the linearization point of the operation.

The NBBST is an easy example because the function  $F_I$  from the proof of Theorem 22 is essentially an identity function. We show a more complicated example with Harris's linked list in Appendix F. With an appropriately defined  $F_I$ , the proof structure we used for Theorem 22 works for Michael and Scott's queue [42], Harris's linked list [35], Natarajan and Mittal's BST [43], and chromatic BSTs [18]. For these algorithms, we need to slightly modify the sequential, read-only operations to make them solo queries. The mapping  $F_A$  is always defined to be the standard mapping from sequential to abstract state and the key property to prove is that  $F = F_A \circ F_I$ .

## C Proof of Theorem 15

*Proof.* We construct  $D_\ell$  from  $D$  as described by Construction 13. We want to show that  $D_\ell$  is a linearizable implementation of the data structure  $D$  with all of its operations in  $Q_D$  and  $L_D$ . We do so by mapping each history  $H_\ell$  of  $D_\ell$  to a history  $H$  of  $D$  in which all solo linearizable queries are run in isolation, and in which all read and CAS operations return the same values as the `readSnapshot`, `vRead` and `vCAS` operations in  $H_\ell$ . Furthermore,  $H_\ell$  and  $H$  will have the exact same high-level history.

Given a history  $H_\ell$  of  $D_\ell$ , we map it to a history  $H$  of  $D$  as follows. (1) For every query operation  $q \in Q_D$  we move all `readSnapshot(h)` operations executed by  $q$  to appear immediately after the `takeSnapshot` that returned  $h$ , in the same order. We then remove the `takeSnapshot`, and replace all `readSnapshot(h)` operations with reads of the corresponding CAS objects of  $D$ . (2) For every `vRead` or `vCAS` operation that appears in  $H_\ell$ , we simply map it to a `read` or `CAS` (respectively) on the corresponding CAS object in  $D$ , without moving it in the history.

Note that by the definition of the versioned CAS object, `vRead` and `vCAS` behave the same as `read` and `CAS` in CAS objects. Furthermore, note that the only operations that are moved in  $H_\ell$  to form  $H$  are `readSnapshot` operations, which do not affect the state of the versioned CAS object they operate on. Thus, all `read` and `CAS` operations in  $H$  return the same values that their corresponding `vRead` and



vCAS operations returned in  $H_\ell$ . Recall from the definition of the versioned CAS object that  $\text{readSnapshot}(h)$  always returns the value of the versioned CAS object it operates on at the time that handle  $h$  was produced. Thus, a read of a CAS object in  $H$  executed at the concurrent state at which the handle  $h$  was produced returns the same value as the  $\text{readSnapshot}(h)$  operation anywhere in the history  $H_\ell$ .

Since  $D$  is a solo linearizable data structure and  $H$  is a legal history of  $D$  in which all solo operations run in isolation,  $H$  is a linearizable history. Since all operations in  $H$  return the same values as they return in  $H_\ell$ ,  $H_\ell$  is also linearizable. Furthermore, we can linearize any operation  $\ell \in L_D$  in  $H_\ell$  at the same step as it linearizes in  $H$  (where we map steps of  $H_\ell$  to steps of  $H$  in the same way as above), and any operation  $q \in Q_D$  at its  $\text{takeSnapshot}$  operation.

To show the required running time bounds, note that operations in  $D$  and operations in  $D_\ell$  access the same number of base objects. The difference in running time for operations in  $L_D$  is strictly due to the time it takes to access the versioned CAS object for vCAS and vRead operations. By Theorem 2, this amounts to constant overhead. Operations  $q \in Q_D$  execute one  $\text{takeSnapshot}$  operation, which takes constant time, and then replace every read they would do in the implementation of  $D$  with a  $\text{readSnapshot}(h)$  where  $h$  is the handle returned by the  $\text{takeSnapshot}$ . By Theorem 2, the running time of each  $\text{readSnapshot}(h)$  is proportional to the number of successful vCAS operations on that object since  $h$  was produced. Note that all such vCAS operations on all versioned CAS objects that the query accesses are concurrent with the query itself. Thus, we get our desired time bounds.  $\square$

## D Relationship of Strong Linearizability to Direct Linearizability

Strong linearizability was introduced by Golab, Higham and Woelfel [34] to provide a stronger guarantee that permits reasoning about concurrent executions that involve randomness. At first glance, it seems that this condition might be what is required for our approach to be applicable. We show here that strong linearizability is *not* comparable to direct linearizability (defined in Definition 17), which is the property required for our approach.

Intuitively, an implementation is strongly linearizable if linearization points for each operation can be chosen as the execution proceeds, without needing to know what happens later in the execution. (See [34] for the formal definition; the informal definition will suffice for this discussion.)

We first show that strong linearizability does not imply direct linearizability. Consider a non-deterministic ADT  $A$  stores a single bit and provides the following two operations. `Write-random-bit`, which sets the bit to either 0 or 1, non-deterministically, and returns *ack*). `Read` simply

returns the current value of the bit. Let  $D$  be an implementation that delays the choice of the random bit written by a `write-random-bit` until the first subsequent `read` operation. More precisely,  $D$  uses a writable CAS object  $X$  with three possible states,  $\perp, 0, 1$ . A `write-random-bit` operation simply writes  $\perp$  into  $X$ . A `read` does a  $\text{CAS}(X, \perp, \text{random}(0, 1))$  and returns the new value if the CAS is successful, or the old value if the CAS is unsuccessful. Since each operation performs only one shared-memory access in  $D$ , that access must serve as the linearization point of the operation. It is easy to see that this linearization is correct. Thus, linearization points can be determined without having to know what happens later in the execution. In other words,  $D$  is strongly linearizable. However,  $D$  is not directly linearizable: when  $X$  is in state  $\perp$ , there is no abstract state that can be used as the value of the abstraction function  $F$ . If  $F(\perp) = 0$ , then an execution in which the subsequent read returns 1 would violate Definition 16. A similar problem arises if  $F(\perp) = 1$ .

Indeed, our approach would fail if we tried to apply it to  $D$ : if a  $\text{takeSnapshot}$  is performed between a `write-random-bit` and the first subsequent `read`, reading the snapshot would yield  $\perp$ , and it would be impossible to conclude what state of  $A$  this corresponds to. Thus, strong linearizability is not a sufficient condition for our approach to be applicable.

Next, we show that direct linearizability does not imply strong linearizability. The snapshot ADT [4] stores a vector of values and allows processes to update components of the vector or perform a `scan` that reads the whole vector atomically. The classic implementation of [4] implements a snapshot using an array of values (with associated timestamps to avoid ABA problems). Updates are performed by writing the new value to the appropriate location in the array and changing its timestamp. A `scan` reads the array repeatedly until getting identical results twice. This implementation is not strongly linearizable [34], but it is directly linearizable: the abstraction function simply strips the timestamps from the elements stored in the array to get the state of the ADT.

## E Examples

Our first example focuses on the concurrent queue implementation by Michael and Scott presented in [42]. We will call this implementation MS-QUEUE. Thus, we have  $D = \text{MS-QUEUE}$ , and  $A$  is the abstract data type of a FIFO queue that stores integers and supports the operations `enqueue` and `dequeue`.

We start by describing how MS-QUEUE works. MS-QUEUE [42] implements the queue using a simply-linked list of `Node` objects, each storing a key and a `next` pointer pointing to the next `Node`. Two pointers, called `Head` and `Tail`, point to the first and the last element of the list that implements the queue, respectively. The first `Node` of the list is always a dummy `Node`. Thus, the elements of the queue are the keys of the `Nodes` starting from the second `Node` of the list up until its last `Node`. Initially, the list contains just the dummy `Node`,

whose key can be arbitrary and its `next` pointer is equal to NULL. At each point in time, the list contains those elements that have been inserted in the queue and have not yet been deleted, in the order of insertion. It also contains the last element that has been dequeued as the first element of the list (i.e., as the dummy Node).

To insert a key  $k$  in the queue, a process  $q$  has to call `Enqueue(k)`. `Enqueue` first allocates a new Node  $nd$  with key  $k$  and its `next` field equal to NULL. It then reads `Tail` and checks whether the `next` field of the Node it points to is equal to NULL. If this is so, `Tail` points to the last element of the queue, and `Enqueue` attempts to insert  $nd$  after this Node using a CAS. If this CAS is successful, then  $q$  performs one more CAS trying to update `Tail` to point to  $nd$ . Otherwise, some other process managed to insert its own Node as the next to the last one, so  $q$  has to retry. If the Node pointed to by `Tail` does not have its `next` field equal to NULL, then some process has managed to insert its own Node as the next Node to the one pointed to by `Tail` but it has not yet updated `Tail` to point to this Node (i.e., `Tail` is falling behind). To ensure lock-freedom, whenever  $q$  discovers that `Tail` is falling behind, it helps by updating `Tail` to point to the last Node of the list, before it restarts its own operation.

A process  $q$  executing `Dequeue`, reads both `Head` and `Tail`. If they both point to the same Node and the `next` field of this Node is NULL, then the queue is empty (it contains just the dummy Node) so `false` is returned. If they point to the same Node, but the `next` field of this Node is not NULL, then `Tail` is falling behind, so  $q$  has to help by performing a CAS to update `Tail` to point to the last Node of the queue before it retries its own operation. If `Head` and `Tail` do not point to the same Node, `Dequeue` reads the key of the second Node of the list and performs a CAS in an effort to update `Head` to point to this Node. If the CAS is successful, `Dequeue` completes by returning the key that it read (and the Node from where it read this key becomes the dummy Node). Otherwise,  $q$  restarts the execution of `Dequeue`.

In MS-QUEUE, the `Head` pointer always points to the first element of the list, whereas the `Tail` pointer always points either to the last or to the second last pointer of the list. This implies that whenever the `next` pointer of the last element of the list changes to point to a newly inserted Node, `Tail` points to the last Node of the list. Moreover, whenever `Head` is updated, `Tail` does not point to the first element of the list. These properties and the way helping is performed make it possible to assign linearization points to the queue operations in two different ways. A `Dequeue` is linearized when `Head` is updated to point to the list Node whose element the `Dequeue` returns. An `Enqueue` can be linearized either at the point the `next` field of the last Node changes to point to the newly inserted Node, or it can be linearized when the `Tail` pointer changes to point to the newly inserted Node (notice that the latter change might not be performed

by the same process that initiated the `Enqueue`). Note that whenever `Dequeue` interferes with `Enqueue`, i.e., whenever there is just one element in the queue, `Dequeue` first updates `Tail` to point to the last Node (if needed) and then performs the deletion. In this way, `Head` is never ahead of `Tail` and therefore the linearization point of an `Enqueue` always precedes the linearization point of the `Dequeue` that deletes the element that the `Enqueue` inserted in the list. (Note that this is true for both ways of assigning linearization points.) It is also not hard to prove that the list is always connected, and the Nodes are appended at the end of the list, and that they are extracted from the beginning of it, in the order defined by the sequence of the linearization points assigned to `Enqueue` operations.

Note that the way we choose to assign linearization points allows us to determine the annotations for the executions of MS-QUEUE (in a straightforward way). Note that both linearization schemes, assign the linearization point of an operation at the point in time that a concrete CAS is executed, i.e. each linearization point is assigned at the point that an internal actions of the MS-QUEUE I/O automaton occurs. This allows us to come up with an abstraction **function** in each case.

Figures 4 and 5 show how to implement two kinds of read-only queries on top of MS-QUEUE using versioned CAS objects. The first, called `peekEndPoints`, returns the values of the first and the last element in the queue. The second implements `scan`, i.e., it returns a set containing the keys of all queue Nodes.

To implement these queries, we have to perform the simple changes to MS-QUEUE described in Section 4. We call the resulting algorithm VER-QUEUE. In VER-QUEUE, `Head` and `Tail` are versioned CAS objects storing references to VNode objects whose `val` field points to the first and the last Node of the list, respectively. Similarly, the `next` field of each Node is a versioned CAS object storing a reference to a VNode object that contains the pointer to the next Node in the queue. The code for `Enqueue` and `Dequeue` remains unchanged but every read to `Head`, `Tail` or to the `next` field of a Node has to be replaced with an invocation of `vRead` (on the same object). Similarly, every CAS on each of these objects, has to be replaced with a `vCAS` (on the same object with the same old and new values). We remark that all versioned CAS objects are associated with a single camera object  $S$ . A `takeSnapshot` is invoked on this camera object at the beginning of every query.

`peekEndPoints` starts by performing a `takeSnapshot` and storing the resulting handle into a local variable `ts`. Finally, it executes `readSnapshot(ts)` to read both `Head` and `Tail` and returns the values it read.

A `scan` first executes `takeSnapshot` to get a handle `ts`, and also reads `Head` and `Tail` using `readSnapshot(ts)`. Then, it executes a while loop to traverse the list starting from the node pointed to by the value read in `Head` until the node

pointed to by the value read in `Tail`. It uses a set to collect the pointers of the nodes it traverses (other than the first one) and returns this set at the end. On each node, it calls `readSnapshot(ts)` to move to the next node. This ensures that updates that occurred in the list after the point that the global timestamp was increased will not be included in the set.

## E.1 A Versioned Concurrent BST Implementation based on the NBBST

We start with a brief, informal description of the concurrent binary search tree (BST) implementation provided in [26], which we will call NBBST. NBBST implements a leaf-oriented tree, i.e., a tree that represents a set whose elements are the keys stored only in the leaf nodes of the tree. The tree is full, i.e., every internal node has exactly two children. Moreover, the tree satisfies the following sorting property: for every internal node  $v$  with key  $K$ , the key of every node in the left subtree of  $v$  is smaller than  $K$ , whereas every node in the right subtree of  $v$  has key larger than or equal to  $K$ .

NBBST supports three operations, `Insert( $k$ )`, `Delete( $k$ )`, and `Find( $k$ )`, where  $k$  is a key. All three operations start by calling `Search( $k$ )`, a routine that searches for  $k$  by following the standard BST searching algorithm. `Search` returns a pointer  $l$  to the leaf that it arrives, a pointer  $p$  to its parent node, and a pointer  $gp$  to the grandparent of this leaf. `Find` simply checks whether the leaf node returned by `Search` contains key  $k$ . If it does, it returns `true`, otherwise `false` is returned.

In its sequential version, `Insert` replaces the leaf that the `Search` arrives at with a BST of three nodes, two leaves containing the key of the node pointed to by  $l$  and the newly-inserted key, and an internal node containing the larger key among the keys of the two leaves. The replacement is performed by switching the appropriate pointer of  $p$  from  $l$  to the root of this BST. `Delete` essentially performs the inverse action: it switches the appropriate child pointer of  $gp$  from  $p$  to the sibling of the node pointed to by  $l$ , thus replacing a part of the tree that is comprised of three nodes (one of which is the leaf to be deleted) with one node, namely the sibling of the node to be deleted.

To avoid synchronization problems, NBBST uses CAS to apply a change to a child pointer of a node. Such a CAS is called a *child CAS*. Moreover, it flags a node when its child pointer is to be changed, and unflags it after the change of the child pointer has been performed. These two types of CAS are called *flag CAS*, and *unflag CAS*, respectively. Thus, NBBST uses flagging to “lock” a node (in a non-blocking manner) whose child pointer is to be changed. NBBST marks an internal node when the node is to be deleted. It does so by executing a *mark CAS*. A marked node remains marked forever. To implement flagging and marking, each node has a two-bit status field, which can have one of the following four values: `CLEAN`, `FLAG` for insertion, `FLAG` for deletion, or

`MARK`. A flag or mark CAS can succeed only if it is applied on a node whose status is `CLEAN`. If a flag CAS fails, the process that performed the flag CAS retries the execution of its operation by starting it from scratch. If the operation is a `Delete` and the flag CAS succeeds but the mark CAS fails, then the process first unflags  $gp$ , using a *backoff CAS*, and then retries the execution of its operation.

To ensure lock-freedom, each process executing an operation records in an *Info* object all the information needed by other processes to complete the operation. A pointer to such an object is stored together with the status field of a node (and they are manipulated atomically). A process  $q$  that fails to flag or mark a node helps the operation that has already flagged or marked the node to complete (by reading the necessary information in the *Info* object pointed to by the status field of the node). Then,  $q$  restarts its own operation. This ensures that a single operation cannot repeatedly block another operation from making progress. Thus, lock-freedom is ensured.

For NBBST, it is proved that each node a `Search( $k$ )` visits was in the tree, on the search path for  $k$ , at some time during the `Search`. `Search( $k$ )` is linearized at the point when the leaf it returns was on the search path for  $k$ . The `insert` and `delete` operations that return `false` are linearized at the same point as the `Search` they perform. Every `insert` or `delete` operation that returns `true` has a unique successful child CAS and the operation is linearized at that child CAS.

Figures 6 and 7 show how we can modify NBBST to support queries using versioned CAS objects. We call the resulting algorithm VER-BST. They also provide pseudocode for `RangeSum( $a, b$ )`, a query that returns the set of those keys in the implemented set that are larger than or equal to  $a$  and smaller than or equal to  $b$ .

In VER-BST, the `child[LEFT]` or `child[RIGHT]` field of each internal Node  $v$  is a versioned CAS object storing a reference to a *VNode* object that contains the pointer to the left or right child, respectively, of  $v$  in the tree. Moreover, every read of the `child[LEFT]` or `child[RIGHT]` field of a Node is replaced with an invocation of `vRead` (on the same object). Similarly, every CAS on each of these fields, is replaced with a `vCAS` (on the same object with the same old and new values). We remark that the `status` field of a Node does not have to be a versioned CAS object, as queries simply ignore the flag and mark signs on the Nodes. Notice that all versioned CAS objects are paired with the same camera on which a `takeSnapshot` is invoked at the beginning of the execution of every query.

`RangeSum( $a, b$ )` first performs a `takeSnapshot`. Then, it calls the recursive function `RSTraverse` which traverses part of the tree to perform the required calculation. Pseudocode for `RangeSum` is provided in Figure 7.

In VER-BST, linearization points can be assigned to `insert` and `delete` operations the same way as in NBBST. A query



```

2531 1 // View both ends of the queue
2532 2 <Value, Value> peekEndpoints () {
2533 3   Node* HNode, TNode;
2534 4   int ts = TS.takeSnapshot();
2535 5   HNode = Head.readSnapshot(ts);
2536 6   TNode = Tail.readSnapshot(ts);
2537 7   if (HNode != TNode) {
2538 8     HNode = HNode->next.readSnapshot(ts);
2539 9     return <HNode->val, TNode->val>; }
2540 10  return <⊥, ⊥>;
2541 11 }
2542
2543 13 List<Node*> SCAN () {
2544 14   List<Node*> Result;  \\ initially empty
2545 15   int ts = TS.takeSnapshot();
2546 16   Node* q = Head.readSnapshot(ts);
2547 17   Node* last = Tail.readSnapshot(ts);
2548 18   while (q != last) {
2549 19     q = q->next.readSnapshot(ts);
2550 20     Result.append(q); }
2551 21   return Result;
2552 22 }
2553

```

Figure 4. Two Example Query Operations for VER-QUEUE.

is linearized at the linearization point of the `takeSnapshot` it invokes on Line 2.

## F Solo queries for Harris's Linked List

Each node in the Harris linked list contains a `key` field and a `next` field. The `next` field stores a pointer that is potentially marked, indicating that the node containing this `next` field has been logically deleted. A state of the Harris linked list consists of a set of nodes and a pointer to the first node in the linked list.

The technique we use from constructing solo is similar to the technique we applied to the NBBST in Section B.2.1. Just like the NBBST, Harris's linked list implements an ordered set ADT. First, we define  $F_A$  to be the standard mapping from sequential linked lists to ordered sets which basically maps a linked list to the set of keys that appear in its nodes. If  $q_I$  is a read-only, sequential linked list operation implementing the abstract query  $q_A$ , then by the correctness of  $q_I$ , we know that  $q_I(S) = q_A(F_A(S))$  for all sequential states  $S$ . Just like in Section B.2.1, we use  $q_I(S)$  to denote the return value of  $q_I$  when run on state  $S$ . Next, we define a mapping  $F_I$  from concurrent states to sequential linked list states such that  $F = F_A \circ F_I$  is an abstraction function. For each sequential, read-only linked list operation  $q_I$  implementing the abstract query  $q_A$ , we show how to modify  $q_I$  into a read-only operation  $q$  for the Harris linked list such that for all reachable concurrent states  $C$ ,  $q(C) = q_I(F_I(C))$ . Once we have these facts, it is fairly

```

2586 23 class Node {
2587 24   Value val;
2588 25   VersionedCAS <Node*> next;
2589 26   Node(Value v, Node* n) :
2590 27     {val = v; next = n;}
2591 28 };
2592
2593 30 class Queue {
2594 31   VersionedCAS <Node*> Head, Tail;
2595 32   Camera TS;
2596
2597   /*
2598   Same code except replacing each
2599   read of Head, Tail or the next
2600   field of a Node with readSnapshot
2601   and replacing each CAS on these
2602   variables with a vCAS
2603   */
2604   ...
2605
2606 43 };
2607

```

Figure 5. Node representation and Code updates for Enqueue and Dequeue in MS-QUEUE.

straight-forward to complete the proof. From the equalities we've proven  $q(C) = q_I(F_I(C)) = q_A(F_A(F_I(C))) = q_A(F(C))$  for all reachable concurrent states  $C$ , so by Observation 20,  $q$  can be added to Harris's linked list as a solo query.

In Harris's original paper [35], he linearizes successful `insert` operations when the node being inserted gets connected to the data structure and successful `delete` operations when the node being deleted gets marked for deletion (i.e. when the node gets logically deleted, not physically deleted). We need to define  $F_I$  so that the abstraction function  $F_A \circ F_I$  is consistent when these linearization points. To compute  $F_I(C)$ , we physically delete (i.e. unlink) all the logically deleted nodes from  $C$  and return the resulting linked list as the sequential state. Using an argument similar to the proof of Proposition 18, we can show that  $F = F_A \circ F_I$  is an abstraction function for Harris's linked list.

Now we show how to transform  $q_I$  into  $q$ . Let  $q_I$  be a read-only, sequential linked list operation implementing the abstract query  $q_A$ . To construct  $q$ , whenever  $q_I$  reads the next pointer of a node, change it to call the `getNext` function implemented in Figure 8. This function basically skips over any marked nodes and returns the next unmarked node. This effectively ignores logically deleted nodes. Therefore, running  $q$  on a reachable concurrent state  $C$  has the same effect as running  $q_I$  on  $F_I(C)$ . Plugging all this into the proof framework we specified earlier shows that  $q$  can be added to Harris's linked list as a solo query.

```

2641 1 class InternalNode { // subclass of Node
2642 2     Key key;
2643 3     HelpRec hr;
2644 4     array VersionedCas<Node *> child[LEFT,RIGHT]
2645 5     Node(Key k, HelpRec up, Node* lc, Node* rc) :
2646 6     {key = k; hr = up; child[LEFT] = lc; child[RIGHT] = rc;}
2647 7 };
2648
2649 9 class BST {
265010     Node* Root;
265111     Camera TS;
2652
265313     // Same code except replacing read of child[LEFT] or child[RIGHT] field
265414     // of a Node with readSnapshot and CAS on them with vCAS
265515     // appropriate initialization is necessary
265616     ...
2657
2658
265918 };

```

Figure 6. Node representation and Code updates for insert and delete in NBBST.

```

2663 1 Integer RangeSum(Key a, Key b) {
2664 2     int ts = TS.takeSnapshot();
2665 3     return RSTraverse(Root, ts, a, b); }
2666
2667
2668 5 Integer RSTraverse(Node *nd, int ts, Key a, Key b) {
2669 6     if (nd points to a leaf node and nd->key is in [a,b]) return nd->key;
2670 7     else {
2671 8         if (a <= nd->key) {
2672 9             return RSTraverse(nd->child[RIGHT].readSnapshot(ts), ts, a,b); }
267310         else if (b < nd->key) {
267411             return RSTraverse(nd->child[LEFT].readSnapshot(ts), ts, a, b); }
267512         else {
267613             return RSTraverse(nd->child[LEFT].readSnapshot(ts), ts, a, b) +
267714                 RSTraverse(nd->child[RIGHT].readSnapshot(ts), ts, a, b); }
267815     }
267916 }

```

Figure 7. An Example Query Operation for VER-BST.

```

2683 1 struct Node { Key key; Node* next; }
2684
2685 3 Node* getNext(Node* node) {
2686 4     Node* n = node->next;
2687 5     while(n != NULL && is_marked(n->next))
2688 6         n = unmark(n->next);
2689 7     return n; }
2690
2691
2692
2693
2694
2695

```

Figure 8. Implementation of the getNext operation for Harris Linked List.

```

2751 1  using Value = Node*;
2752 2  class Camera {
2753 3      int timestamp;
2754 4      Camera() { timestamp = 0; }
2755 5      int takeSnapshot() {
2756 6          // same as in VerCAS}
2757 7      Value invalidNextv = new Node();
2758 8      int TBD = -1;
2759 9      class Node {
276010          /* other fields of
276111          Node struct of D */
276212          ...
276313          Value nextv; // initially invalidNextv
276414          int ts; // initially TBD };
276515      class OptVersionedCAS {
276616          Value Head;
276717          Camera* S;
276818          OptVersionedCAS(Value v, Camera* s) {
276919              S = s;
277020              Head = v;
277121              if(Head != NULL) {
277222                  initNextv(Head);
277323                  initTS(Head); } }
277424          void initNextv(Value n) {
277525              if(n->nextv == invalidNextv)
277626                  CAS(&n->nextv, invalidNextv, NULL);}
277727          void initTS(Value n) {
277828              if(n->ts == TBD) {
277929                  int curTS = S->timestamp;
278030                  CAS(&n->ts, TBD, curTS); } }

```

```

31  Value OptreadSnapshot(int ts) {
32      Value node = Head;
33      if(node != NULL) initTS(node);
34      while(node != NULL && node->ts > ts)
35          node = node->nextv;
36      return node; }
37  Value OptvRead() {
38      Value head = Head;
39      if(node != NULL) initTS(head);
40      return head; }
41  bool OptvCAS(Value oldV, Value newV) {
42      Value head = Head;
43      if(node != NULL) initTS(head);
44      if (head != oldV) return false;
45      if (newV == oldV) return true;
46      CAS(&n->nextv, invalidNextv, NULL);
47      if(CAS(&Head, head, newV)) {
48          initTS(newV);
49          return true; }
50      else {
51          // Head can't be NULL
52          initTS(Head);
53          return false; } }

```

**Figure 9.** Linearizable implementation of a versioned CAS object without indirection. Major differences between this and Figure 1 are highlighted.

## G Direct versioned CAS Algorithm

Here we consider the correctness and give pseudocode for the optimization that avoid indirection. Consider two versioned CAS objects  $O_1$  and  $O_2$ . Roughly speaking, since all nodes are recorded-once, every vCAS operation on any versioned CAS object stores a distinct value. This means that every time a vCAS is executed (on any versioned CAS object), it writes a pointer to a newly allocated node. Thus, the only way for a node  $nd$  other than the last in the version list of  $O_1$ , to appear in the version list of  $O_2$ , is if a pointer to  $nd$  were used as the initial value of  $O_2$ . Hence  $nd$  is the last node in  $O_2$ 's version list. We argue that no invocation of `OptreadSnapshot` on a versioned CAS object  $O$  traverses the `nextv` pointer of the last node in the version list of  $O$ . These imply that the version lists of versioned CAS objects behave as if they are disjoint. In particular, we never have to store `nextv` pointers for two

different version lists in the same node. Based on the above arguments, we can prove that  $D_{opt}$  is linearizable.

We present code in Figure 9.
